# Supplementary material for: Nutri-ATLAS: Embodied Agent for Tabulated Lookup and Assistance for Smarter nutrition
Source: arXiv:2609.32803 source file (2026-09-26)
Supplement: Supplementary file 1 [file appendix.tex]

\appendix

\section{Additional Embodied Evaluation Results}
\label{app:additional_results}


\begin{figure*}[t]
  \centering
  \includegraphics[width=\textwidth]{figures/gantt_three_levels.png}
  \caption{\textbf{Tool-call sequences for 15 benchmark tasks across three difficulty levels.} 
  Each row represents one task; colored blocks indicate individual tool invocations within a single model turn, ordered from left to right. Simple tasks involve single-step actions such as navigation or object lookup. Intermediate tasks require multi-step spatial reasoning, such as scene scanning or cross-room retrieval. Challenging tasks require longer plans with conditional navigation and memory-based object queries.}
  \label{fig:tool_sequence}
\end{figure*}


\begin{table*}[!t]
\centering
\begin{tabular}{|l|c|c|c|c|c|c|c|c|}
\hline
\textbf{Nutrients} & \multicolumn{2}{c|}{\textbf{Carbohydrate}} & \multicolumn{2}{c|}{\textbf{Protein}} & \multicolumn{2}{c|}{\textbf{Fat}} & \multicolumn{2}{c|}{\textbf{Energy}} \\
\hline
Metrics & Accuracy (\%) & MAE & Accuracy (\%) & MAE & Accuracy (\%) & MAE & Accuracy (\%) & MAE \\
\hline
Baseline & $45.5$ & $26.6$ & $73.5$ & $7.00$ & $67.8$ & $9.99$ & $50.8$ & $\mathbf{154.6}$ \\
\hline
BM25~\cite{robertson2009probabilistic} & $46.6$ & $30.0$ & $67.4$ & $9.11$ & $67.8$ & $10.38$ & $43.6$ & $221.4$ \\
\hline
Dense Retrieval~\cite{lewis2020retrieval} & $46.4$ & $26.7$ & $65.2$ & $8.37$ & $63.1$ & $10.69$ & $41.3$ & $192.3$ \\
\hline
Nutri-ATLAS RAG & $\mathbf{52.8}$ & $\mathbf{17.3}$ & $\mathbf{78.6}$ & $\mathbf{6.99}$ & $\mathbf{69.4}$ & $\mathbf{9.32}$ & $\mathbf{51.7}$ & $188.1$ \\
\hline
\end{tabular}
\caption{Nutri-ATLAS performance on NutriBench v2 using Qwen3.5-9B with 4-bit quantization across retrieval-augmented generation configurations with Recall@5. Accuracy denotes the fraction of predictions within the predefined tolerance of the ground truth. MAE is reported in grams for macronutrients and kcal for energy. BM25 uses sparse keyword retrieval, Dense Retrieval uses embedding-based nearest-neighbor search, and Dense + GAT further augments dense retrieval with graph-based nutritional re-ranking.}
\label{tab:qwen_results}
\end{table*}


% \section{Example Interaction Log from the Nutri-ATLAS System}
% \label{app:example_log}

% This appendix provides a representative interaction log from an experiment conducted with the proposed Nutri-ATLAS system. The example demonstrates the full pipeline, including user query interpretation, nutrition recommendation generation, embodied kitchen search, environment scanning, and final feedback to the user.

% \subsection{User Request and Nutrition Recommendation}

% \noindent\textbf{User:} \textit{``i have taken an apple for dinner, what should i take for breakfast''}

% \vspace{0.5em}
% \noindent\textbf{System Internal Log:}
% \begin{verbatim}
% [nutrition] eaten="an apple", 
%     meal_type=dinner, next=breakfast
% [nutrition] Initializing NutriAssistant 
%     (loading embeddings + DB)...
% [nutrition] NutriAssistant ready.
% \end{verbatim}

% \vspace{0.5em}
% \noindent\textbf{System Response:}

% Based on your nutritional needs, here's a breakfast recommendation:

% \begin{quote}
% \textbf{Smoked Provolone \& Blue Crab Toast with a Pear Slice}

% This meal is designed to balance your macros while addressing your protein and fat needs.

% \textbf{Ingredients \& Portions:}
% \begin{itemize}
%     \item \textbf{Protein Source:} \textbf{Smoked Provolone Cheese} (sliced, smoked) -- Approx.\ 30g (about 2--3 slices)
%     \item \textbf{Protein Source:} \textbf{Blue Swimming Crab Meat} (pasteurized, refrigerated) -- Approx.\ 35g (about $1/4$ cup)
%     \item \textbf{Carb Source:} \textbf{Pear} (raw, with skin) -- Approx.\ 1 medium pear (150g)
%     \item \textbf{Fat Source (Optional):} Add 1 teaspoon of olive oil or a few slices of avocado if needed
% \end{itemize}

% \textbf{Approximate Nutritional Breakdown:}
% \begin{itemize}
%     \item \textbf{Protein:} $\sim$24g--26g
%     \item \textbf{Fat:} $\sim$9g--11g
%     \item \textbf{Carbohydrates:} $\sim$35g--38g
%     \item \textbf{Calories:} $\sim$240--260 kcal
% \end{itemize}

% \textbf{Why this works for you:}
% \begin{enumerate}
%     \item \textbf{Fixes the Protein Gap:} Your current intake is very low in protein. This meal brings you to over 25g, supporting muscle maintenance.
%     \item \textbf{Adds Healthy Fats:} The provolone cheese provides the necessary fat content, improving satiety.
%     \item \textbf{Balanced Carbs:} The pear provides moderate carbohydrates without excessive spikes.
% \end{enumerate}

% \textit{Note:} If crab meat is unavailable, it can be substituted with an additional 15g of Monterey Jack cheese to maintain the protein and fat balance.
% \end{quote}

% \subsection{Embodied Search Request}

% \noindent\textbf{User:} \textit{``can you looking for those food for me?''}

% \vspace{0.5em}
% \noindent\textbf{System Internal Log:}
% \begin{verbatim}
% [list_landmarks] listing all landmarks
% [get_current_detected_objects] called
% [navigate_to_landmark] navigating to: kitchen
% [spin_robot] rotating 120.0°
% [get_current_detected_objects] called
% [spin_robot] rotating 120.0°
% [get_current_detected_objects] called
% [spin_robot] rotating 120.0°
% [get_current_detected_objects] called
% [get_detected_objects] called

% [navigate_to_landmark] navigating to: 
%     (-4.85, -3.07)
% [spin_robot] rotating 120.0°
% [get_current_detected_objects] called
% [spin_robot] rotating 120.0°
% [get_current_detected_objects] called
% [spin_robot] rotating 120.0°
% [get_current_detected_objects] called
% [get_detected_objects] called

% [nutrition] eaten="an apple", 
%     meal_type=dinner, next=breakfast
% \end{verbatim}

% \subsection{Final System Feedback After Kitchen Search}

% \noindent\textbf{System Response:}

% \begin{quote}
% I've completed a full 360$^\circ$ scan of the kitchen area and checked the refrigerator. Unfortunately, I couldn't find any of the specific ingredients from the breakfast recommendation (Smoked Provolone cheese, Blue Swimming Crab, or fresh pears) in the kitchen or refrigerator.

% Here's what I found in the kitchen:
% \begin{itemize}
%     \item Refrigerator (empty of the needed items)
%     \item Oven, microwave, bowls, and some kitchen accessories
%     \item A potted plant and vase
% \end{itemize}

% \textbf{What you can do:}
% \begin{enumerate}
%     \item \textbf{Check your pantry or other storage areas} -- Sometimes ingredients are kept in cabinets or other rooms.
%     \item \textbf{Consider alternative options} -- If the specific items are unavailable, you might:
%     \begin{itemize}
%         \item use what is already available,
%         \item visit a grocery store or market, or
%         \item request a different breakfast option based on accessible ingredients.
%     \end{itemize}
% \end{enumerate}

% The system then offered the following follow-up options:
% \begin{itemize}
%     \item Search other rooms (e.g., bedroom or living room) for food items
%     \item Provide alternative breakfast recommendations based on commonly available foods
%     \item Help navigate to a nearby grocery store if available
% \end{itemize}
% \end{quote}
